# Supplementary material for: BWS: Best Window Selection Based on Sample Scores for Data Pruning across Broad Ranges
Source: arXiv:2406.03057 source file (2024-06-05)
Supplement: Supplementary file 1 [file classwise.tex]

\color{blue}

BWS algorithm \ref{alg1} provides window subset that results in best accuracy at proxy task(the kernel ridge regression problem) among interested window subsets.
However, the search space of window subsets are quite restricted because BWS only checks window subsets consisting of data whose scores are in $[s, s+w]\%$ for each class.
In detail, we select data within $[s, s+w]\%$ for each class.
We extend the pool of checking window subsets, by selecting best window subsets 
However, we check that selecting data 
In this section, we propose

\color{black}
